# Supplementary material for: Plasmonic Metasurfaces with Structural Chirality and Pseudo-Chirality for Enhanced Circular Dichroism and Enantiomeric Recognition
Source: arXiv:2508.00730 source file (2025-08-01)
Supplement: Supplementary file 1 [file Supporting_information.pdf]

# Supporting Information

## Plasmonic Metasurfaces with Structural Chirality and Pseudo-Chirality for Enhanced Circular Dichroism and Enantiomeric Recognition

*Giovanna Palermo, Bryan Guilcapi, Radoslaw Kolkowski, Alexa Guglielmelli, Dante M. Aceti, Liliana Valente, Joseph Zyss, Lucia Petti*, Giuseppe Strangi*.*

### S1. Electromagnetic simulations

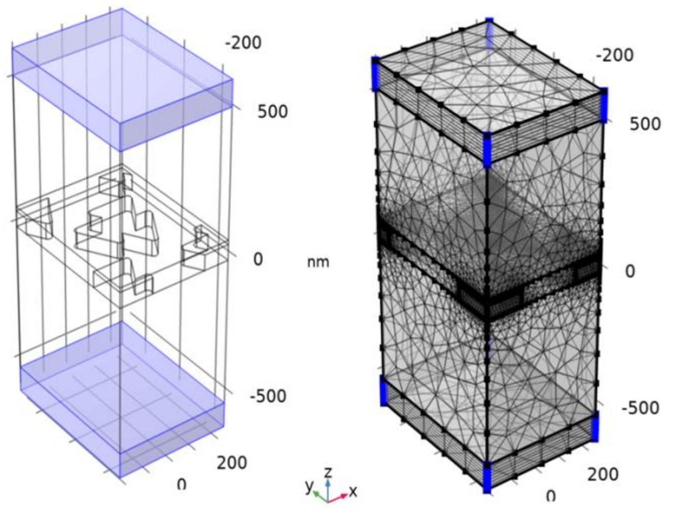


**Figure S1:** 3D COMSOL model of the metasurface used for optical simulations. Left: geometry of the unit cell, including the chiral nanostructure embedded between substrate and superstrate domains. Right: corresponding finite element mesh used for the full-field electromagnetic calculations.

To simulate the metasurface in COMSOL Multiphysics, we created a 3D model consisting of a parallelepiped of wavelength-dependent height.

The parallelepiped is constituted by 4 regions: starting from the bottom: i) the glass substrate with a refractive index $n_{glass}$ = 1.52; ii) the gold nanostructures with optical constants taken from Refs. [1-2], iii) the chiral layer, and iv) the upper medium, which is assumed to be water ($n_{H2O}$ = 1.333). To create a wave diffusion environment, an input and an output port were used, to simulate the incidence from top (+z) to bottom (-z) at a specific angle θ. To ensure the infinity conditions in the (x, y) plane, the Periodic Boundary Conditions (PBCs) were applied to the surfaces along the (x, y) directions of the blocks. To simulate the repeated single unit cell, the Floquet periodicity was used. In addition to the PBCs, Perfectly Matched Layers (PMLs) were introduced into the simulated system to implement an absorbing

boundary condition at the block extremes. The equations were solved by discretizing the model using the built-in automatic geometry-sensitive meshing algorithm under an “extremely-fine” mesh setting – see Figure S1.
The circular polarization of the impinging radiation can be suitably selected by considering the following amplitude for the electric field: (1,1i,0) for the Left-handed circular polarized light (LCP) and (1,-1i,0) for the Right-handed circular polarized light (RCP).
The transmittance through the structure is obtained from the built-in Scattering Matrix coefficients.
To simulate the chiral layer, the COMSOL equations were altered in the equation view of the physics setup as reported in the following table:

| | | | |
|---|---|---|---|
| ewfd.Dx | epsilon0_const*(ewfd.epsilonrxx*ewfd.Ex)+i*(xi(lambda)*ewfd.Bx) | C/m² | Electric displacement field, x component |
| ewfd.Dy | epsilon0_const*(ewfd.epsilonryy*ewfd.Ey)+i*(xi(lambda)*ewfd.By) | C/m² | Electric displacement field, y component |
| ewfd.Dz | epsilon0_const*(ewfd.epsilonrzz*ewfd.Ez)+i*(xi(lambda)*ewfd.Bz) | C/m² | Electric displacement field, z component |
| ewfd.Hx | (1/mu0_const)*(ewfd.murinvxx*ewfd.Bx)+i*(xi(lambda)*ewfd.Ex) | A/m | Magnetic field, x component |
| ewfd.Hy | (1/mu0_const)*(ewfd.murinvyy*ewfd.By)+i*(xi(lambda)*ewfd.Ey) | A/m | Magnetic field, y component |
| ewfd.Hz | (1/mu0_const)*(ewfd.murinvzz*ewfd.Bz)+i*(xi(lambda)*ewfd.Ez) | A/m | Magnetic field, z component |
| ewfd.dHdtx | ((ewfd.murinvxx*ewfd.dBdtx+ewfd.murinvxy*ewfd.dBdty+ewfd.murinvxz*ewfd.dBdtz)/mu0_const)-(ewfd.omega*xi(lambda)*ewfd.Ex) | A/(m·s) | Magnetic field, time derivative, x component |
| ewfd.dHdty | ((ewfd.murinvyy*ewfd.dBdty+ewfd.murinvyx*ewfd.dBdtx+ewfd.murinvyz*ewfd.dBdtz)/mu0_const)-(ewfd.omega*xi(lambda)*ewfd.Ey) | A/(m·s) | Magnetic field, time derivative, y component |
| ewfd.dHdtz | ((ewfd.murinvzz*ewfd.dBdtz+ewfd.murinvzx*ewfd.dBdtx+ewfd.murinvzy*ewfd.dBdty)/mu0_const)-(ewfd.omega*xi(lambda)*ewfd.Ez) | A/(m·s) | Magnetic field, time derivative, z component |

## S2. Line profiles of the AFM and SNOM measurements

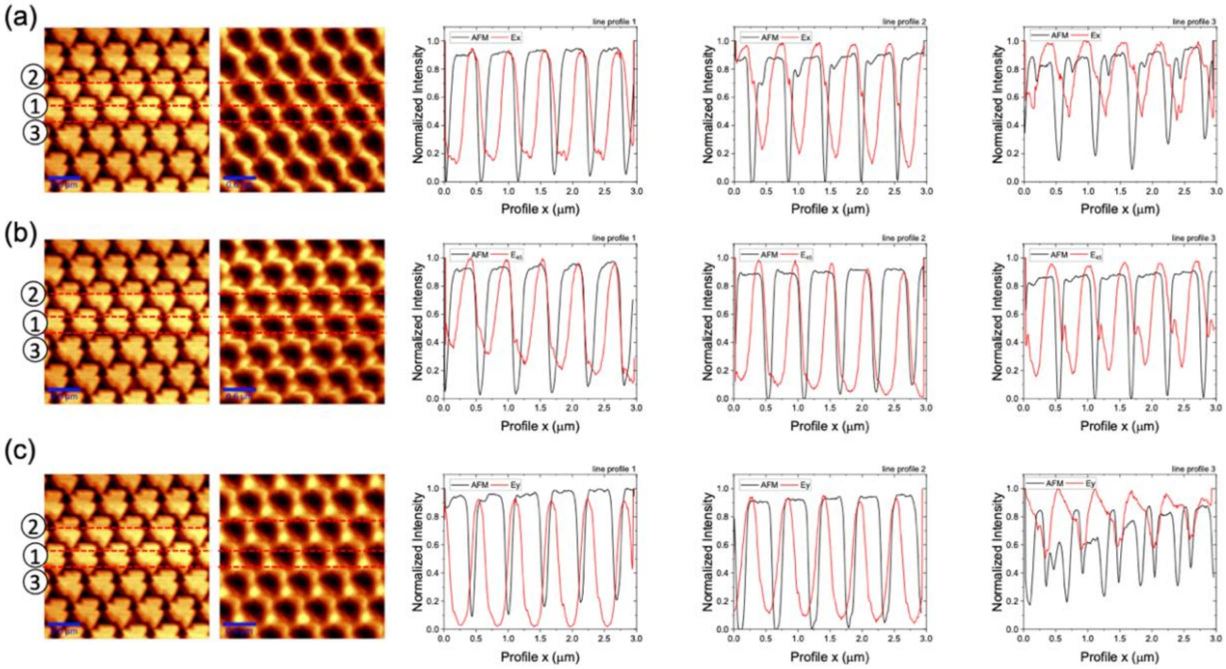


**Figure S2**: Comparison between the AFM topography and the near-field optical field distributions acquired via SNOM for three different polarizations of the incident light: (a) $E_x$-polarization , (b) $E_{45°}$-polarization, and (c) $E_y$-polarization.

The first two columns show AFM and SNOM images of the same area of the plasmonic metasurface, respectively. The three dashed red lines labeled 1, 2, and 3 indicate the line profiles extracted to compare the structural features with the localized optical field distribution. The following columns display the normalized intensity profiles along each line, highlighting the overlap between surface morphology (black) and optical hot-spots (red).

The intensity peaks of the optical field do not exactly coincide with the topographic features, indicating localized plasmonic effects influenced by both the geometry and the incident field orientation. These observations confirm the crucial role of structural anisotropy in modulating the local optical response of the metasurface.

## S3. Far-field analysis of the metasurface with air as surrounding medium

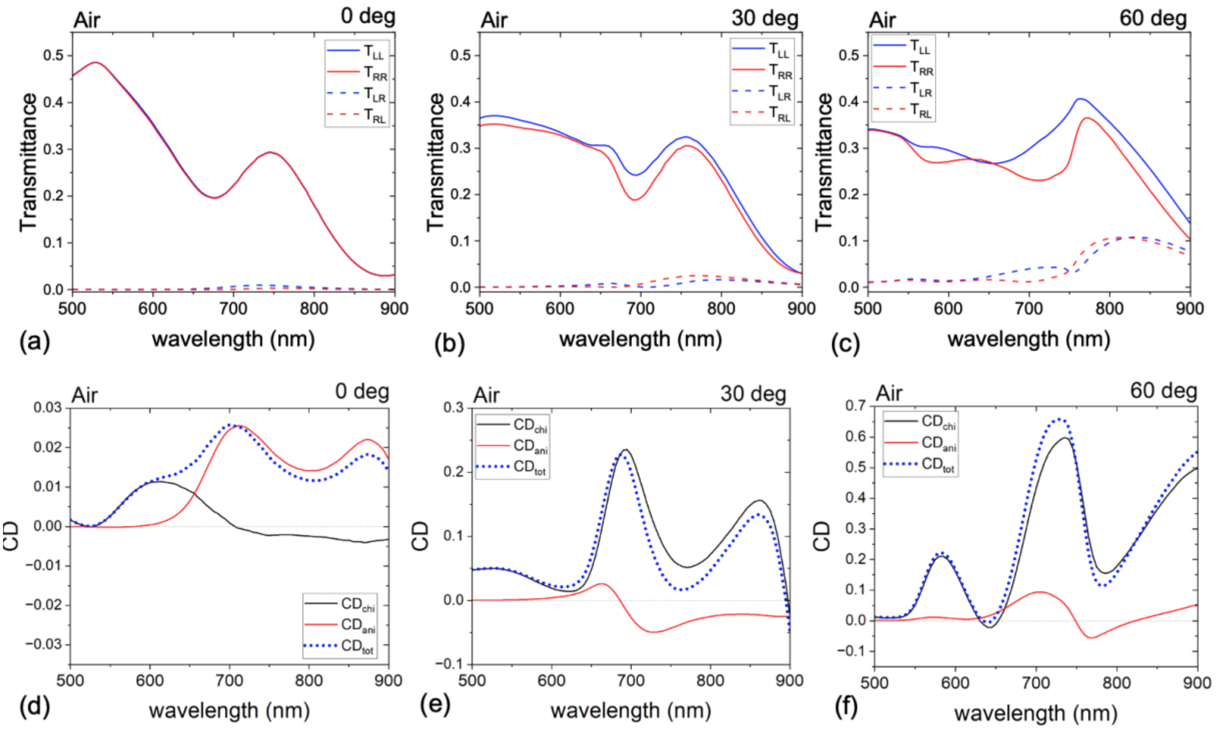


**Figure S3**: Transmittance and circular dichroism (CD) spectra calculated for the metasurface under oblique incidence in air at different angles: 0° (a, d), 30° (b, e), and 60° (c, f). (a–c) show the transmission coefficients for circularly polarized light: co-polarized components $t_{LL}$, $t_{RR}$ and cross-polarized components $t_{LR}$. (d–f) show the corresponding decomposition of the circular dichroism into chiral ($CD_{chi}$, black line) and anisotropic ($CD_{ani}$, red line) contributions, with the total CD ($CD_{tot}$) shown as blue open circles.

This figure highlights the strong dependence of the metasurface's chiroptical response on the angle of incidence. At normal incidence (0°), the total CD is affected by anisotropic chiral effects. As the angle increases, chirality begins to play a more significant role, leading to a large enhancement of the total CD signal. The clear separation of chiral and anisotropic contributions allows for a better understanding of the origin of the observed optical activity and the design of metasurfaces with tailored chiroptical functionalities.

## S4. Role of the substrate in the chiroptical response

To isolate the impact of the substrate on the observed chiroptical effects, we performed simulations in two configurations: a) the actual experimental geometry with air as superstrate and glass ($n$ = 1.52) as substrate, and b) a hypothetical symmetric configuration with air on both sides of the metasurface (i.e., without substrate). As shown in Figure S4, the presence of the glass substrate significantly alters the spectral shape and amplitude of the circular dichroism components. In the asymmetric case (a), both the anisotropic contribution ($CD_{ani}$) and the chiral component ($CD_{chi}$) are clearly visible and contribute

constructively to the total CD signal ($CD_{tot}$), resulting in a broadband positive response with peaks exceeding 0.025. The non-zero $CD_{chi}$ demonstrates the intrinsic-chiral effects enabled by the presence of the substrate.

In contrast, the symmetric case (b) reveals a markedly different behavior. Here, the total CD spectrum is dominated almost entirely by the anisotropic contribution, with $CD_{chi}$ remaining close to zero across the entire spectral range. This confirms that in the absence of vertical symmetry breaking (i.e., when no refractive index contrast is present along the z-direction), the structure does not support any net chiral optical response under circularly polarized illumination. The resulting CD response arises solely from in-plane birefringence ($CD_{ani}$).

These results confirm that the substrate plays a critical role in enabling and enhancing the chiral optical behavior of the metasurface. By breaking mirror symmetry along the propagation direction, it activates intrinsic chiral effects that would otherwise be forbidden in fully symmetric environments.

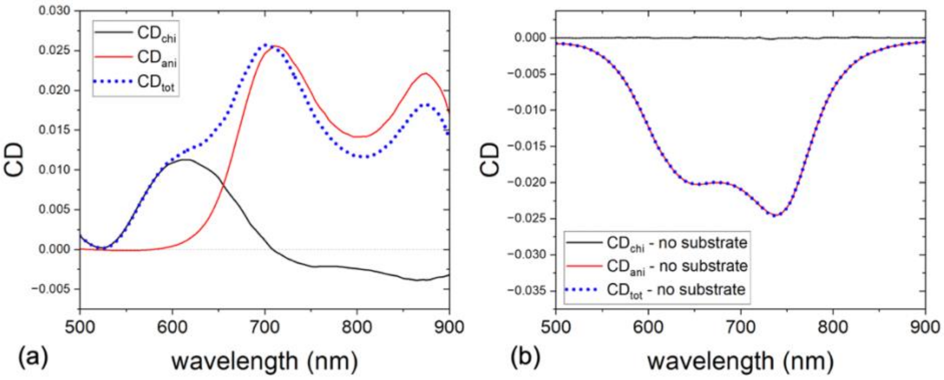


**Figure S4**: Comparison of the chiroptical response of the metasurface with and without substrate. (a) Simulated circular dichroism spectra showing the chiral ($CD_{chi}$, black), anisotropic ($CD_{ani}$, red), and total ($CD_{tot}$, blue dotted) contributions in the realistic configuration with air as superstrate and glass as substrate.
(b) Corresponding CD components for the symmetric configuration with air on both sides (no substrate).

## S5. Calculation of the chiral parameter ξ

To estimate the chiral response of molecular dielectrics used in our study, we followed the formalism described by Govorov et al., [3] and Kelly et al. [4] which provides a wavelength-dependent expression for the chiral parameter ξ, a local quantity that defines the strength and handedness of optical chirality in a material. The value of ξ can be computed from the following expression:

$$\xi(\lambda) = \beta_c \left( \frac{1}{\frac{hc}{\lambda} + \frac{hc}{\lambda_0} + i\Gamma_{12}} + \frac{1}{\frac{hc}{\lambda} - \frac{hc}{\lambda_0} + i\Gamma_{12}} \right)$$

Here, $\beta_c$ is an intrinsic molecular coefficient, $\lambda$ is the probe wavelength, $\lambda_0$ is the resonance absorption wavelength of the chiral molecule, $\Gamma_{12}$ is the linewidth, and $hc$ is the product of Planck's constant and the speed of light, expressed in eV μm. In our case, the constants used were:

$hc$ = 1.23984 eV μm

$\Gamma_{12}$ = 0.4 eV

$\beta_c$ = 4.1 $10^{-4}$ eV

$\lambda_0$= 0.450 μm

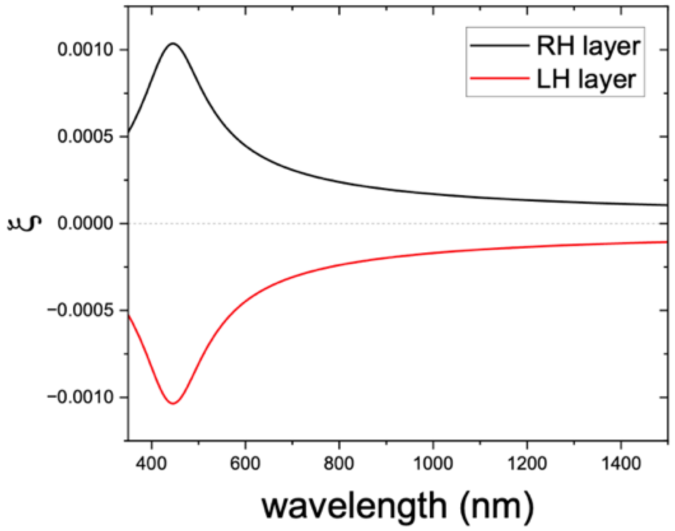


**Figure S5**: ξ magnitude for a Left-Handed (LH) (ξ < 0) and a Right-Handed (RH) (ξ > 0) molecular dielectric layer.

## S6. Evaluation of the enhancement of the optical chiral density

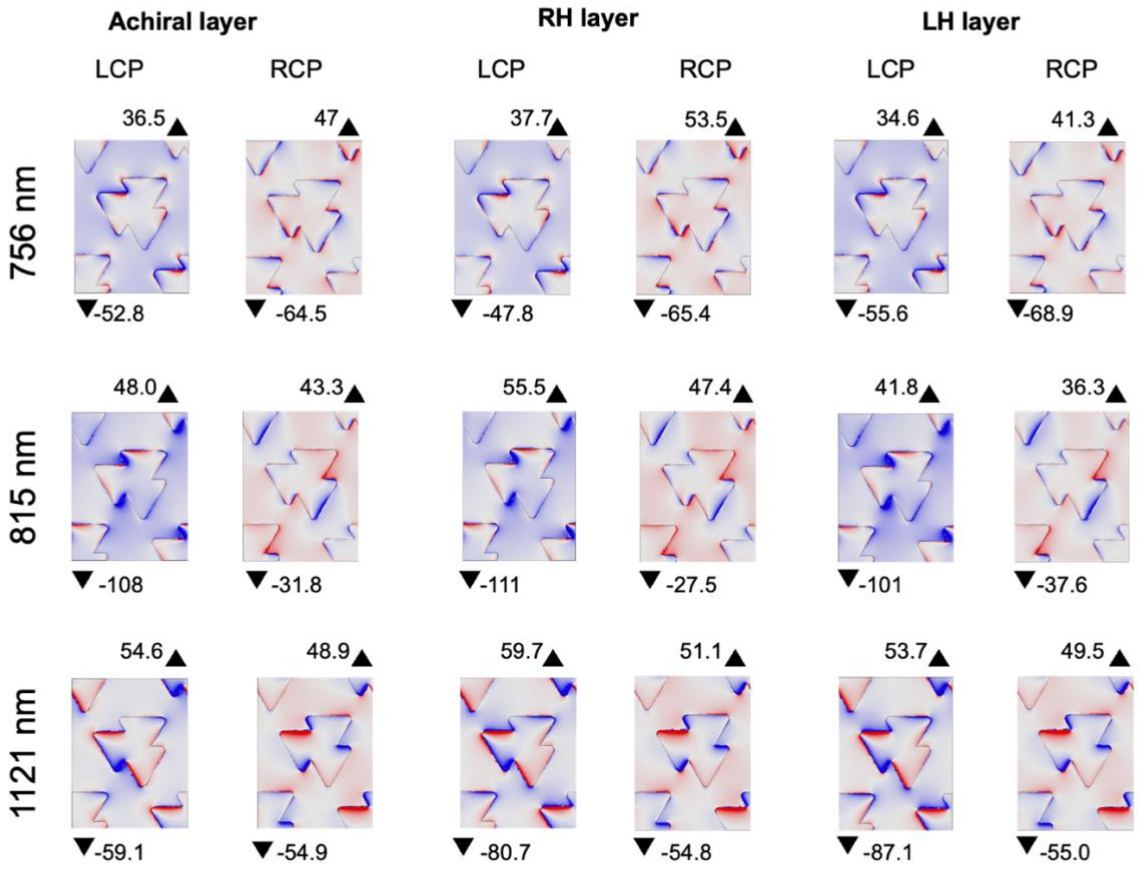


**Figure S6.** Normalized optical chirality density $C/|C_0|$, evaluated at three wavelengths: 756 nm, 815 nm, and 1121 nm. The maximum and minimum values are reported above and below each map.

References:


1. Johnson, P. B., & Christy, R. W. (1972). Optical constants of the noble metals. *Physical Review B*, *6*(12), 4370.
2. Polyanskiy, M. N. (2024). Refractiveindex. info database of optical constants. *Scientific Data*, *11*(1), 94.
3. Govorov, A. O. & Fan, Z. (2012) Theory of chiral plasmonic nanostructures comprising metal nanocrystals and chiral molecular media. *ChemPhysChem*.13, 2551–60.
4. Kelly, C., Khosravi Khorashad, L., Gadegaard, N., Barron, L. D., Govorov, A. O., Karimullah, A. S., & Kadodwala, M. (2018). Controlling metamaterial transparency with superchiral fields. *ACS Photonics*, 5(2), 535-543.
